# Supplementary material for: Exploring and Exploiting Decision Boundary Dynamics for Adversarial Robustness
Source: arXiv:2302.03015 source file (2023-04-15)
Supplement: Supplementary file 1 [file tab_L2_moreEps.tex]

% \begin{table}[!htbp]
% \centering
% \noindent\begin{tabular}{lSSSSSS}
% \centering
% % & \multicolumn{3}{c}{$L_2$} & \multicolumn{3}{c}{$L_\infty$} \\
% % \cmidrule(r){2-4}\cmidrule(l){5-7}
% Defense & {Clean} & {$\epsilon=0.5$}  & {$\epsilon=1$}  & {$\epsilon=1.5$} & {$\epsilon=2$} \\
% \midrule
% AT & {$88.38 \pm 0.23$} & {$65.29 \pm 0.21$} & {$1 \pm 0.21$} & {$1 \pm 0.17$} & {$1 \pm 0.17$} & \\
% TRADES & {$87.05 \pm 0.01$} & {$67.92 \pm 0.11 (70.00 \pm 0.05$)}  & {$1 \pm 0.11$} & {$1 \pm 0.08$} & {$1 \pm 0.04$}   \\
% MMA & {$88.62 \pm 0.14$} & {$65.02 \pm 0.23$} & {$1 \pm 0.23$} & {$1 \pm 0.08$} & {$41.48 \pm 0.21$}    \\
% \midrule
% Ours & {$87.25 \pm 0.05$} & {$67.96 \pm 0.04$} &  {$1 \pm 0.13$} & {$1 \pm 0.14$} & {$1 \pm 0.14$}   \\
% \bottomrule

% \end{tabular}
% \caption{\small{Clean and robust accuracy on CIFAR-10 under $L_2$ attack}}
% \label{table: performance_L2_more_eps}
% \end{table}

\begin{table}[!htbp]
\centering
\noindent
% \caption{\small{Clean and robust accuracy on CIFAR-10 under $L_2$ attack under AA and PGD. Note that the robust accuracy under AA is lower and thus is a more accurate estimate of the robustness. }}
\resizebox{\textwidth}{!}{\begin{tabular}{lSSSSSSSSSS}
\centering
& & \multicolumn{2}{c}{$\epsilon=0.5$} & \multicolumn{2}{c}{$\epsilon=1$} & \multicolumn{2}{c}{$\epsilon=1.5$} & \multicolumn{2}{c}{$\epsilon=2$} \\
\cmidrule(r){3-4}\cmidrule(l){5-6}\cmidrule(l){7-8} \cmidrule(l){9-10}
Defense & {Clean} & {AA}  & {PGD} & {AA}  & {PGD} & {AA}  & {PGD} & {AA}  & {PGD}\\
\midrule
AT & {$88.38 \pm 0.23$} & {$65.29 \pm 0.21$} & {$66.94 \pm 0.14$}  & {$33.71 \pm 0.16$} & {$36.82 \pm 0.14$} & {$11.16 \pm 0.09$} & {$14.86 \pm 0.11$} & {$2.4 \pm 0.17$} & {$4.34 \pm 0.08$} & \\
TRADES & {$87.05 \pm 0.01$} & {$67.92 \pm 0.11 $} & {$69.19 \pm 0.03$} & {$42.08 \pm 0.16$} & {$44.84 \pm 0.23$} & {$19.33 \pm 0.38$} & {$23.01 \pm 0.59$} & {$6.62 \pm 0.16$} & {$9.45 \pm 0.47$} & \\
MMA & {$\boldsymbol{88.40} \pm 0.14$} & {$65.62 \pm 0.23$} & {$66.37 \pm 0.36$} & {$36.54 \pm 0.14$} & {$38.42 \pm 0.21$} & {$14.01 \pm 0.08$} & {$17.52 \pm 0.14$} & {$3.49 \pm 0.10$} & {$6.58 \pm 0.16$} & \\
% MMA-2 & {$85.24 \pm 0.19$} & {$64.88 \pm 0.29$} & {$66.60 \pm 0.24$} & {$42.14 \pm 0.15$} & {$47.85 \pm 0.12$} & {$\boldsymbol{22.18} \pm 0.14$} & {$31.9 \pm 0.18$} & {$\boldsymbol{9.24} \pm 0.08$} & {$19.9 \pm 0.14$} & \\
\midrule
Ours & {$87.25 \pm 0.05$} & {$\boldsymbol{67.96} \pm 0.14$}  & {$68.37 \pm 0.16$}  & {$\boldsymbol{43.48} \pm 0.23$} & {$44.92 \pm 0.21$} & {$\boldsymbol{20.92} \pm 0.12$} & {$22.84 \pm 0.16$} & {$\boldsymbol{6.72} \pm 0.18$} & {$8.95 \pm 0.14$} &  \\
\bottomrule
\end{tabular}}
\caption{\small{Clean and robust accuracy on CIFAR-10 in the $L_2$ setting under AA and PGD. Note that the robust accuracy under AA is a more accurate estimation of the robustness. }}
\label{table: performance_L2_more_eps_app}
\end{table}
