# Supplementary material for: Exploring and Exploiting Decision Boundary Dynamics for Adversarial Robustness
Source: arXiv:2302.03015 source file (2023-04-15)
Supplement: Supplementary file 3 [file tab_L2_ours_ablation.tex]

\begin{table}[!htbp]
\centering
\noindent

\caption{{Clean and robust accuracy of \algoName on CIFAR-10 against AA in the $L_2$ setting.}}
\resizebox{\textwidth}{!}{\begin{tabular}{lSSSSSS}
\centering
{Hyperparameters} & {Clean}  & {$\epsilon=0.5$}  & {$\epsilon=1$} & {$\epsilon=1.5$}  & {$\epsilon=2$} \\
\midrule
{$r_0 = 1, r_1 = 3, g_1 = 0.4, \lambda_c = 1$} & {$\boldsymbol{89.45} \pm 0.12$} & {$63.96 \pm 0.14$}   & {$24.92 \pm 0.22$}  & {$2.89 \pm 0.17$} & {$0.11 \pm 0.03$} & \\

{$r_0 = 1, r_1 = 3, g_1 = 0, \lambda_c = 1$} & {$86.11 \pm 0.12$} & {$66.55 \pm 0.18$}   & {$41.82 \pm 0.16$}  & {$21.73 \pm 0.20$} & {$9.77 \pm 0.13$} & \\

{$r_0 = 2, r_1 = 3, g_1 = 0.4, \lambda_c = 1$} & {$86.18 \pm 0.20$} & {$67.45 \pm 0.19$}   & {$44.28 \pm 0.17$}  & {$21.41 \pm 0.10$} & {$6.83 \pm 0.18$} & \\

{$r_0 = 2, r_1 = 3, g_1 = 0.4, \lambda_c = 2$} & {$87.25 \pm 0.05$} & {$\boldsymbol{67.96} \pm 0.14$}   & {$43.48 \pm 0.23$}  & {$20.92 \pm 0.12$} & {$6.72 \pm 0.18$} & \\

{$r_0 = 2, r_1 = 3, g_1 = 0.4, \lambda_c = 4$} & {$88.77 \pm 0.13$} & {$67.31 \pm 0.17$}   & {$41.74 \pm 0.15$}  & {$18.81 \pm 0.09$} & {$5.76 \pm 0.12$} & \\

{$r_0 = 2, r_1 = 3, g_1 = 0, \lambda_c = 2$} & {$86.19 \pm 0.12$} & {$67.00 \pm 0.18$}   & {$45.16 \pm 0.22$}  & {$24.79 \pm 0.17$} & {$11.61 \pm 0.15$} & \\

{$r_0 = 2, r_1 = 3, g_1 = 0, \lambda_c = 4$} & {$87.15 \pm 0.15$} & {$66.80 \pm 0.22$}   & {$41.88 \pm 0.24$}  & {$20.92 \pm 0.15$} & {$8.50 \pm 0.17$} & \\

{$r_0 = 3, r_1 = 4, g_1 = 0.4, \lambda_c = 2$} & {$85.54 \pm 0.11$} & {$67.69 \pm 0.28$}   & {$\boldsymbol{46.08} \pm 0.19$}  & {$\boldsymbol{25.85} \pm 0.18$} & {$\boldsymbol{11.96} \pm 0.13$} & \\

{$r_0 = 3, r_1 = 4, g_1 = 0.4, \lambda_c = 4$} & {$86.60 \pm 0.07$} & {$66.98 \pm 0.15$}   & {$44.29 \pm 0.10$}  & {$24.21 \pm 0.17$} & {$11.17 \pm 0.09$} & \\
\bottomrule
\end{tabular}}
\label{table: performance_L2_ours_ablation}
\end{table}
