# Supplementary material for: Exploring and Exploiting Decision Boundary Dynamics for Adversarial Robustness
Source: arXiv:2302.03015 source file (2023-04-15)
Supplement: Supplementary file 4 [file tab_Linf_moreEps.tex]

\begin{table}[!htbp]
\centering
\noindent
\caption{\small{Clean and robust accuracy on CIFAR-10 in the $L_\infty$ setting under AA and PGD. Note that the robust accuracy under AA is a more accurate estimation of the robustness. }}
\resizebox{\textwidth}{!}{\begin{tabular}{lSSSSSSSSSS}
\centering
& & \multicolumn{2}{c}{$\epsilon=\frac{8}{255}$} & \multicolumn{2}{c}{$\epsilon=\frac{12}{255}$} & \multicolumn{2}{c}{$\epsilon=\frac{16}{255}$} & \multicolumn{2}{c}{$\epsilon=\frac{20}{255}$} \\
\cmidrule(r){3-4}\cmidrule(l){5-6}\cmidrule(l){7-8} \cmidrule(l){9-10}
Defense & {Clean} & {AA}  & {PGD} & {AA}  & {PGD} & {AA}  & {PGD} & {AA}  & {PGD}\\
\midrule
AT & {$83.25 \pm 0.17$} & {$45.75 \pm 0.15$} & {$49.21 \pm 0.13$}  & {$26.38 \pm 0.14$} & {$30.41 \pm 0.19$} & {$12.34 \pm 0.17$} & {$15.73 \pm 0.12$} & {$4.89 \pm 0.11$} & {$7.35 \pm 0.14$} & \\
TRADES & {$83.54 \pm 0.08$} & {$\boldsymbol{47.18} \pm 0.11$} & {$51.09 \pm 0.01$} & {$29.03 \pm 0.19$} & {$33.96 \pm 0.49$} & {$15.07 \pm 0.11$} & {$19.77 \pm 0.18$} & {$\boldsymbol{6.78} \pm 0.06$} & {$10.17 \pm 0.08$} & \\
MMA & {$84.25 \pm 0.28$} & {$41.48 \pm 0.31$} & {$48.94 \pm 0.21$} & {$23.63 \pm 0.25$} & {$35.41 \pm 0.14$} & {$11.97 \pm 0.20$} & {$25.70 \pm 0.16$} & {$5.11 \pm 0.12$} & {$18.72 \pm 0.18$} & \\
GAIRAT & {$81.31 \pm 0.23$} & {$32.98 \pm 0.11$} & {$58.72 \pm 0.52$} & {$16.19 \pm 0.02$} & {$41.29 \pm 0.52$} & {$6.89 \pm 0.18$} & {$25.16 \pm 0.08$} & {$2.57 \pm 0.07$} & {$12.95 \pm 0.29$} & \\
\midrule
Ours & {$\boldsymbol{85.13} \pm 0.13$} & {$46.47 \pm 0.18$} & {$47.86 \pm 0.22$}  & {$\boldsymbol{29.38} \pm 0.24$} & {$30.19 \pm 0.21$} & {$\boldsymbol{15.14} \pm 0.16$} & {$17.25 \pm 0.12$} & {$6.45 \pm 0.21$} & {$8.23 \pm 0.14$} &  \\
\bottomrule
\end{tabular}}
\label{table: performance_Linf_more_eps_app}
\end{table}
