# Supplementary material for: Exploring and Exploiting Decision Boundary Dynamics for Adversarial Robustness
Source: arXiv:2302.03015 source file (2023-04-15)
Supplement: Supplementary file 5 [file tab_Linf_ours_ablation.tex]

\begin{table}[!htbp]
\centering
\noindent
\caption{{Clean and robust accuracy of \algoName on CIFAR-10 against AA in the $L_\infty$ setting.}}

\resizebox{\textwidth}{!}{\begin{tabular}{lSSSSSS}
\centering
{Hyperparameters} & {Clean}  & {$\epsilon=\frac{8}{255}$}  & {$\epsilon=\frac{12}{255}$} & {$\epsilon=\frac{16}{255}$}  & {$\epsilon=\frac{20}{255}$} \\
\midrule
{$r_0 = \frac{20}{255}, r_1 = \frac{48}{255}, g_1 = 0, \lambda_c = 1$} & {$86.48 \pm 0.17$} & {$44.59 \pm 0.32$}   & {$25.19 \pm 0.27$}  & {$12.17 \pm 0.21$} & {$5.05 \pm 0.19$} & \\

{$r_0 = \frac{20}{255}, r_1 = \frac{48}{255}, g_1 = 0, \lambda_c = 2$} & {$\boldsymbol{87.98} \pm 0.21$} & {$43.38 \pm 0.18$}   & {$23.49 \pm 0.13$}  & {$10.78 \pm 0.17$} & {$4.16 \pm 0.14$} & \\

{$r_0 = \frac{32}{255}, r_1 = \frac{48}{255}, g_1 = 0.4, \lambda_c = 0.5$} & {$84.05 \pm 0.19$} & {$45.90 \pm 0.25$}   & {$28.06 \pm 0.22$}  & {$14.92 \pm 0.14$} & {$6.64 \pm 0.15$} & \\

{$r_0 = \frac{32}{255}, r_1 = \frac{48}{255}, g_1 = 0.4, \lambda_c = 1$} & {$85.13 \pm 0.13$} & {$\boldsymbol{46.47} \pm 0.18$}   & {$\boldsymbol{29.38} \pm 0.24$}  & {$15.14 \pm 0.16$} & {$6.45 \pm 0.21$} & \\

{$r_0 = \frac{32}{255}, r_1 = \frac{48}{255}, g_1 = 0.4, \lambda_c = 2$} & {$86.71 \pm 0.18$} & {$45.76 \pm 0.23$}   & {$26.43 \pm 0.22$}  & {$13.23 \pm 0.19$} & {$5.15 \pm 0.13$} & \\

{$r_0 = \frac{32}{255}, r_1 = \frac{48}{255}, g_1 = 0, \lambda_c = 1$} & {$85.03 \pm 0.18$} & {$45.93 \pm 0.15$}   & {$28.08 \pm 0.20$}  & {$15.53 \pm 0.18$} & {$7.17 \pm 0.14$} & \\

{$r_0 = \frac{32}{255}, r_1 = \frac{48}{255}, g_1 = 0, \lambda_c = 2$} & {$86.87 \pm 0.16$} & {$45.74 \pm 0.20$}   & {$27.40  \pm 0.14$}  & {$14.81 \pm 0.11$} & {$6.58 \pm 0.19$} & \\

{$r_0 = \frac{32}{255}, r_1 = \frac{48}{255}, g_1 = 0, \lambda_c = 3$} & {$87.25 \pm 0.19$} & {$45.62 \pm 0.25$}   & {$26.39 \pm 0.16$}  & {$13.71 \pm 0.16$} & {$5.94 \pm 0.14$} & \\

{$r_0 = \frac{48}{255}, r_1 = \frac{64}{255}, g_1 = 0.4, \lambda_c = 1$} & {$83.64 \pm 0.19$} & {$46.18 \pm 0.16$}   & {$29.21 \pm 0.17$}  & {$\boldsymbol{16.84} \pm 0.20$} & {$\boldsymbol{8.58} \pm 0.15$} & \\

{$r_0 = \frac{48}{255}, r_1 = \frac{64}{255}, g_1 = 0.4, \lambda_c = 2$} & {$85.71 \pm 0.20$} & {$45.64 \pm 0.19$}   & {$28.07 \pm 0.19$}  & {$15.51 \pm 0.09$} & {$7.50 \pm 0.13$} & \\

{$r_0 = \frac{48}{255}, r_1 = \frac{64}{255}, g_1 = 0.4, \lambda_c = 3$} & {$86.26 \pm 0.16$} & {$45.09 \pm 0.27$}   & {$27.39 \pm 0.15$}  & {$15.04 \pm 0.14$} & {$6.94 \pm 0.12$} & \\
\bottomrule
\end{tabular}}
\label{table: performance_Linf_ours_ablation}
\end{table}
